# Supplementary material for: ErrorNet: Learning error representations from limited data to improve vascular segmentation
Source: arXiv:1910.04814 source file (2020-02-02)
Supplement: Supplementary file 1 [file sm.tex]

\documentclass[12pt]{article}
\usepackage{graphicx}
\begin{document}
\begin{figure}[h]
\centering
    \includegraphics[width=0.99\linewidth]{pics/samples.png}
    \caption{Column 1 is the the original fundoscopic image. Column 2 is the ground truth segmentation. Column 3 is the predicted segmentation from the base segmentation module. Column 4 is the predicted segmentation from the base segmentation module with error prediction added.}
\end{figure}
\begin{figure}[h]
\centering
    \includegraphics[width=0.99\linewidth]{pics/improvement_w_arrows.png}
    \caption{Both are segmentations for an fundoscopic image from the ARIA dataset. The image on the left is a segmentation generated by the UNet segmentation model trained on CHASE. The image on the right is the segmentation is generated using ErrorNet and joint training trained on CHASE.}
\end{figure}
\end{document}
